# Supplementary material for: A Cooperative Network Coding Strategy for the Interference Relay Channel
Source: arXiv:1204.2676 source file (2012-05-24)
Supplement: Supplementary file 1 [file appendix.tex]

\appendix
\small

\begin{figure*}[!ht]
\small
\setcounter{MYtempeqncnt}{\value{equation}}
\setcounter{equation}{13}
\begin{eqnarray}
C_{he}-C_{le} &{}={}& k - \mathbb{E}_{B_1, B_2, Y} \left( \log_{2} \left( \frac{\sum_{x \in \chi}P_{Y|X}(Y|x)}{P_{Y|B_1,B_2}(Y|B_1,B_2)} \right) \right) - k + \mathbb{E}_{B_3, B_4, Y} \left( \log_{2} \left( \frac{\sum_{x \in \chi}P_{Y|X}(Y|x)}{P_{Y|B_3,B_4}(Y|B_3,B_4)} \right) \right)
\\
&{=}& \mathbb{E}_{B_1, B_2, Y} \left( \log_{2} P_{Y|B_1,B_2}(Y|B_1,B_2) \right) - \mathbb{E}_{B_3, B_4, Y} \left( \log_{2} P_{Y|B_3, B_4}(Y|B_3, B_4) \right)
\\
&{=}& \sum_{(b_1,b_2)} P(b_1,b_2) \mathbb{E}_{Y|b_1, b_2} \left( \log_{2} P_{Y|B_1,B_2}(Y|b_1,b_2) \right) - \sum_{(b_3,b_4)} P(b_3,b_4) \mathbb{E}_{Y|b_3, b_4} \left( \log_{2} P_{Y|B_3,B_4}(Y|b_3,b_4) \right) \\ 
&{=}& \sum_{(b_1,b_2)} P(b_1,b_2) \mathbb{E}_{Y|b_1, b_2} \left( \log_{2} \sum_{z \in \chi_{b_1,b_2}}P_{Y|X}(Y|z) \right) - \sum_{(b_3,b_4)} P(b_3,b_4) \mathbb{E}_{Y|b_3, b_4} \left( \log_{2} \sum_{z \in \chi_{b_3,b_4}}P_{Y|X}(Y|z) \right) \\
&{=}& C+B
\end{eqnarray}
\setcounter{equation}{\value{MYtempeqncnt}}
\hrulefill
\vspace*{4pt}
\end{figure*}

We use the same notation as in \cite{bicm}. We denote $\chi^+$ the QPSK constellation with energy per symbol $\rho^+ E_s$, $\chi^-$ the QPSK constellation with energy $\rho^- E_s$ and $\chi$ the constellation resulting from the superposition of $\chi^+$ and $\chi^-$. We define the discrete random variables $X^+$, $X^-$ and $X$ as the channel input when the contellation used is $\chi^+$, $\chi^-$ and $\chi$ respectively. We denote the continuous channel output $Y$.

Thus for the QPSK modulation with energy  $\rho^+ E_s$, we have
\begin{equation}
\scriptstyle
C_{qpsk} \left( \rho^+ \frac{E_s}{N_0} \right) \triangleq C_+ = m - \mathbb{E}_{X^+,Y} \left( \log_{2} \left( \frac{\sum_{x \in \chi^+}P_{Y|X^+}(Y|x)}{P_{Y|X^+}(Y|X^+)} \right) \right). 
\label{Cqpsk}
\end{equation}
Replace $\chi^+$ by $\chi^-$ and $X^+$ by $X^-$ for the capacity of the QPSK with energy $\rho^- E_s$, denoted $C_-$.

We also define $B_i$ ($i=1,..,4$) as the value of the i\textsuperscript{th} bit of the label of any constellation point in $\chi$. Thus $C_{he,\alpha}$ and $C_{le,\alpha}$ equal
\begin{equation}
\scriptstyle
k - \mathbb{E}_{B_i, B_j, Y} \left( \log_{2} \left( \frac{\sum_{x \in \chi}P_{Y|X}(Y|x)}{P_{Y|B_i,B_j}(Y|B_i,B_j)} \right) \right), 
\end{equation}
where $(i,j)=(1,2)$ for $C_{he,\alpha}$ and $(i,j)=(3,4)$ for $C_{le,\alpha}$.

We consider the right term, denoted $R$, in the equation of the proposition. In (\ref{Cqpsk}), we develop the $\log_{2}$. Thus $R$ can be written as $A+B+C$. We have
\begin{equation}
\scriptstyle
A = \mathbb{E}_{X^+,Y}(P_{Y|X^+}(Y|X^+)) - \mathbb{E}_{X^-,Y}(P_{Y|X^-}(Y|X^-))
\end{equation}
A simple substitution in the integration gives $A=0$. Then
\begin{equation}
\scriptscriptstyle
B = -\mathbb{E}_{X^+,Y} \left( \log_{2} \sum_{x \in \chi^+}P_{Y|X^+}(Y|x) \right)
\end{equation}
which can also be written as
\begin{equation}
\scriptscriptstyle
B = - \sum_{z \in \chi^+} P_{X^+}(z) \mathbb{E}_{Y|X^+=z} \left( \log_{2} \sum_{x \in \chi^+}P_{Y|X^+}(Y|x) \right)
\end{equation}
In the same way, we have,
\begin{equation}
\scriptscriptstyle
C = \sum_{z \in \chi^-} P_{X^-}(z) \mathbb{E}_{Y|X^-=z} \left( \log_{2} \sum_{x \in \chi^-}P_{Y|X^-}(Y|x) \right)
\end{equation}

We now consider the left term, denoted $L$, in the equation of the proposition.
\normalsize
